# Supplementary material for: Analyzing Machine Learning Workloads Using a Detailed GPU Simulator
Source: arXiv:1811.08933 source file (2019-01-26)
Supplement: Supplementary file 1 [file appendix.tex]

\begin{appendix}

\subsection{IPC Graphs}
% the \\ insures the section title is centered below the phrase: AppendixA

%Chris should add all AerialVision plots we collected
\begin{figure}[h]
\includegraphics[width=\linewidth]{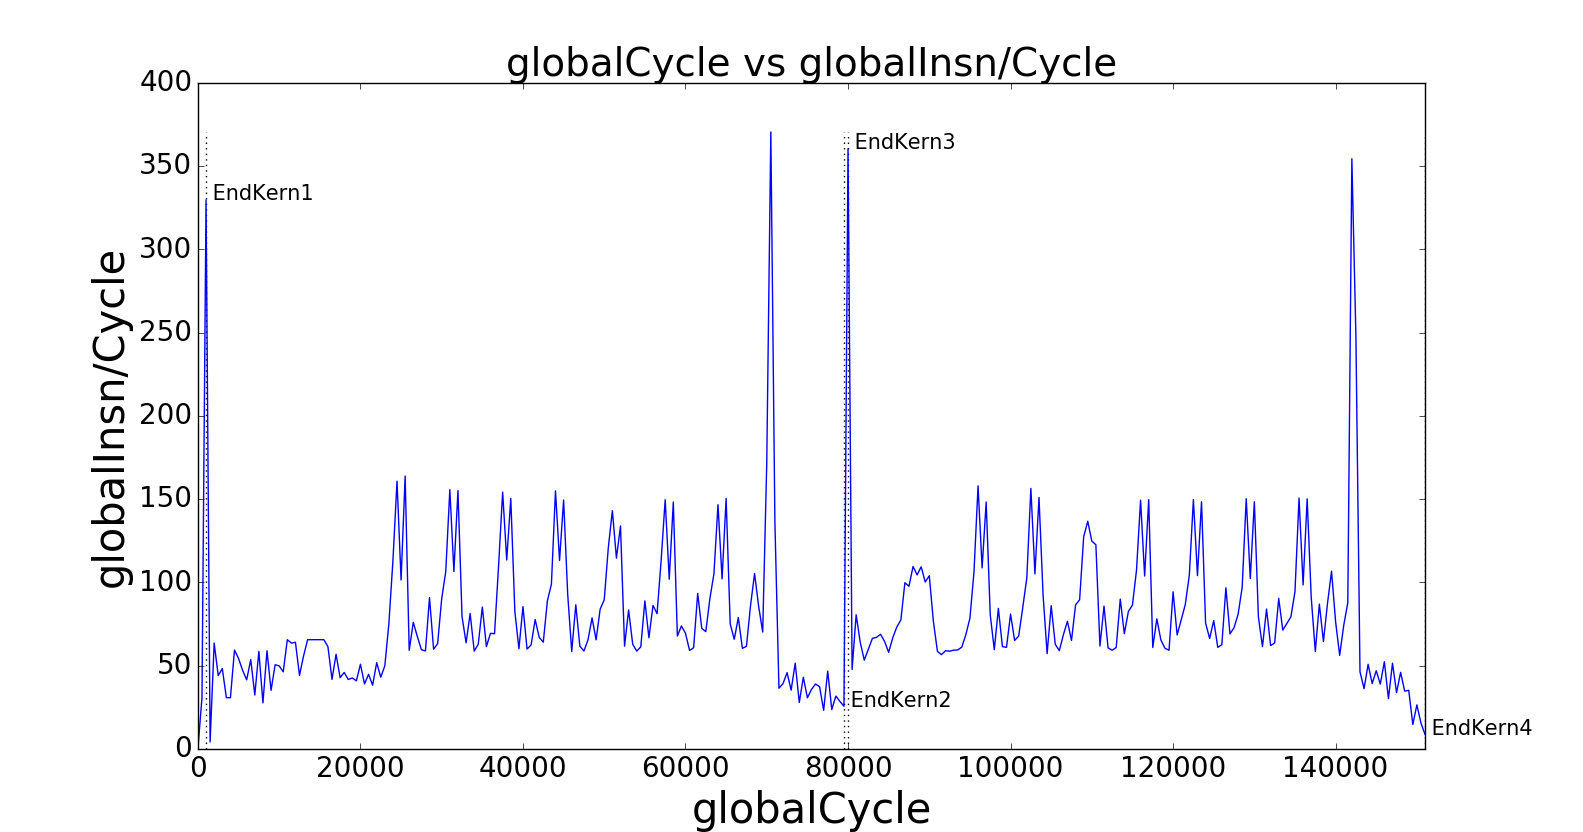}
\caption{Backward Data Convolution (Algorithm 0) Global IPC Plot}
\label{fig:ipc_gemm}
\end{figure}

\begin{figure}[h]
\includegraphics[width=\linewidth]{plots/convdgrad_1/convdgrad_1_gipc.png}
\caption{Backward Data Convolution (Algorithm 1) Global IPC Plot}
\label{fig:ipc_gemm}
\end{figure}

\begin{figure}[h]
\includegraphics[width=\linewidth]{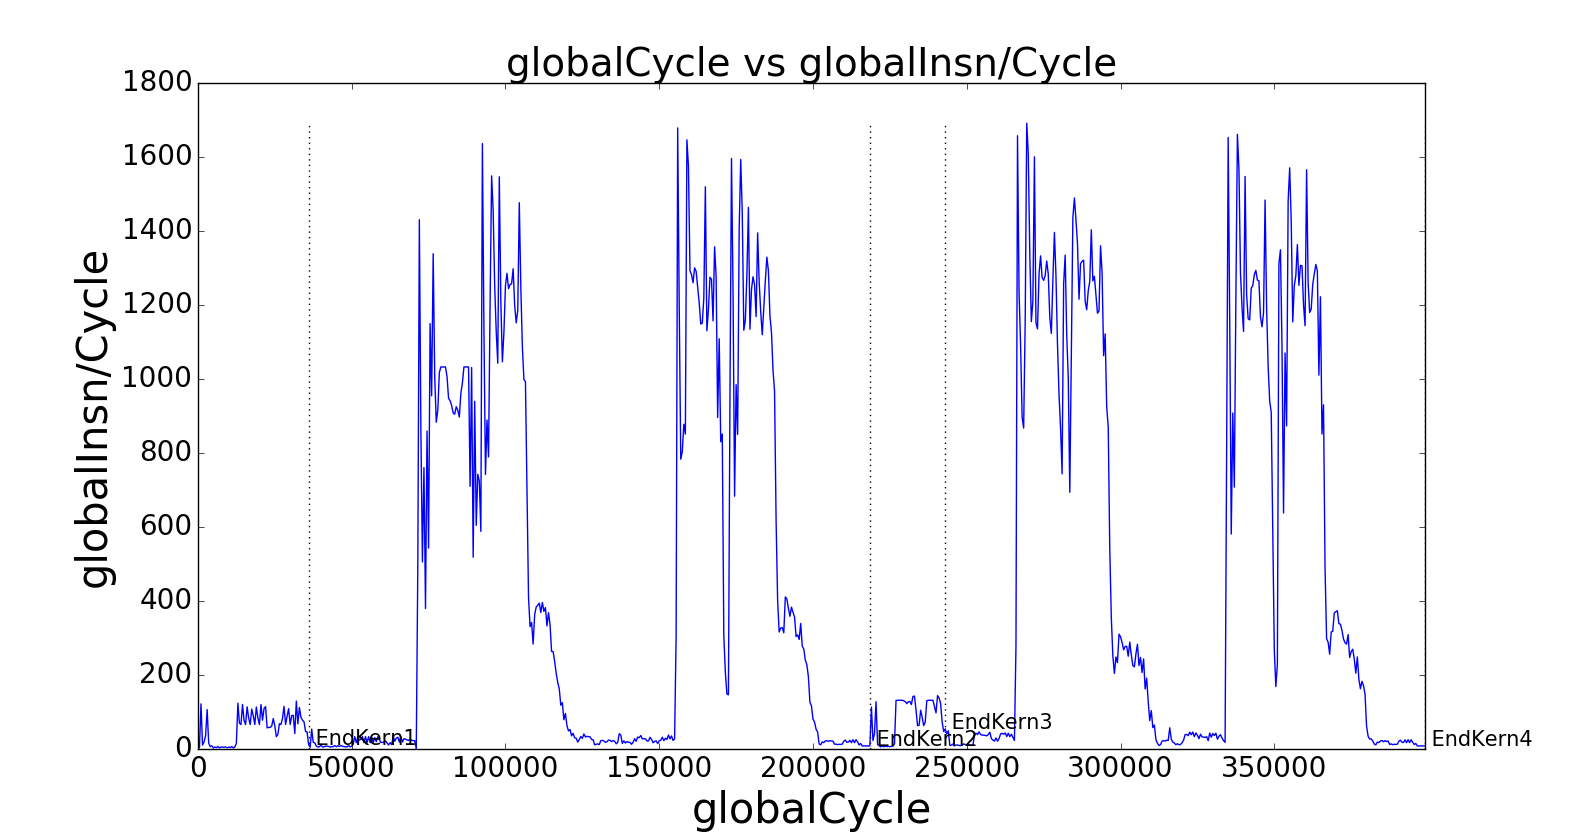}
\caption{Backward Data Convolution (FFT Tiling) Global IPC Plot}
\label{fig:ipc_ffttiling}
\end{figure}

\begin{figure}[h]
\includegraphics[width=\linewidth]{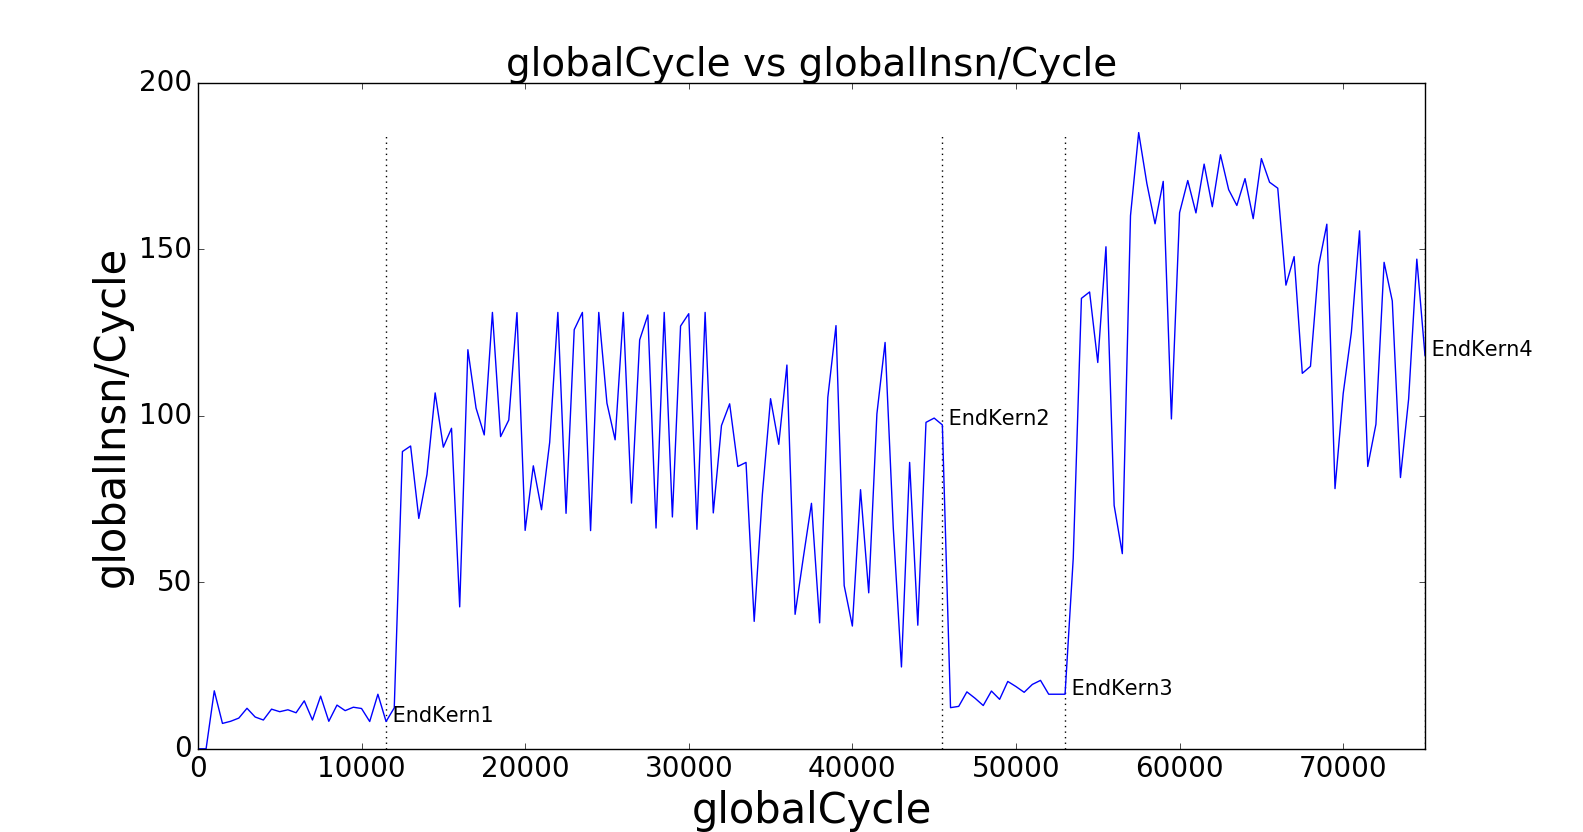}
\caption{Backward Data Convolution (Winograd) Global IPC Plot}
\label{fig:ipc_wwinograd}
\end{figure}

\begin{figure}[h]
\includegraphics[width=\linewidth]{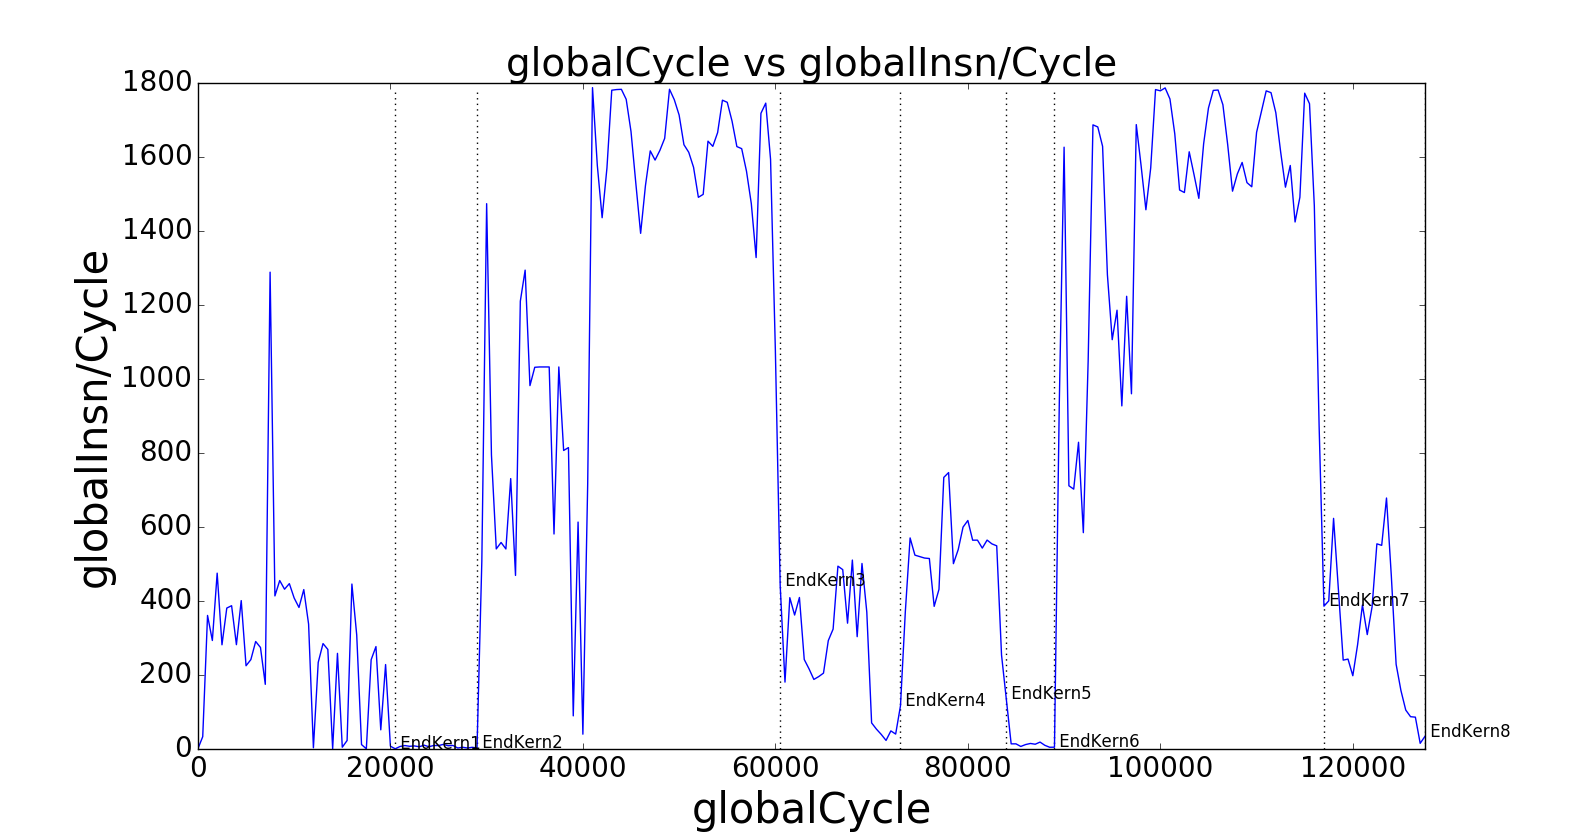}
\caption{Backward Data Convolution (Winograd Non Fused) Global IPC Plot}
\label{fig:ipc_wwinogradnf}
\end{figure}

\begin{figure}[h]
\includegraphics[width=\linewidth]{plots/convfwd_fft/convfwd_fft_gipc.png}
\caption{Forward Convolution (FFT) Global IPC Plot}
\label{fig:dipc_fwdfft}
\end{figure}

\begin{figure}[h]
\includegraphics[width=\linewidth]{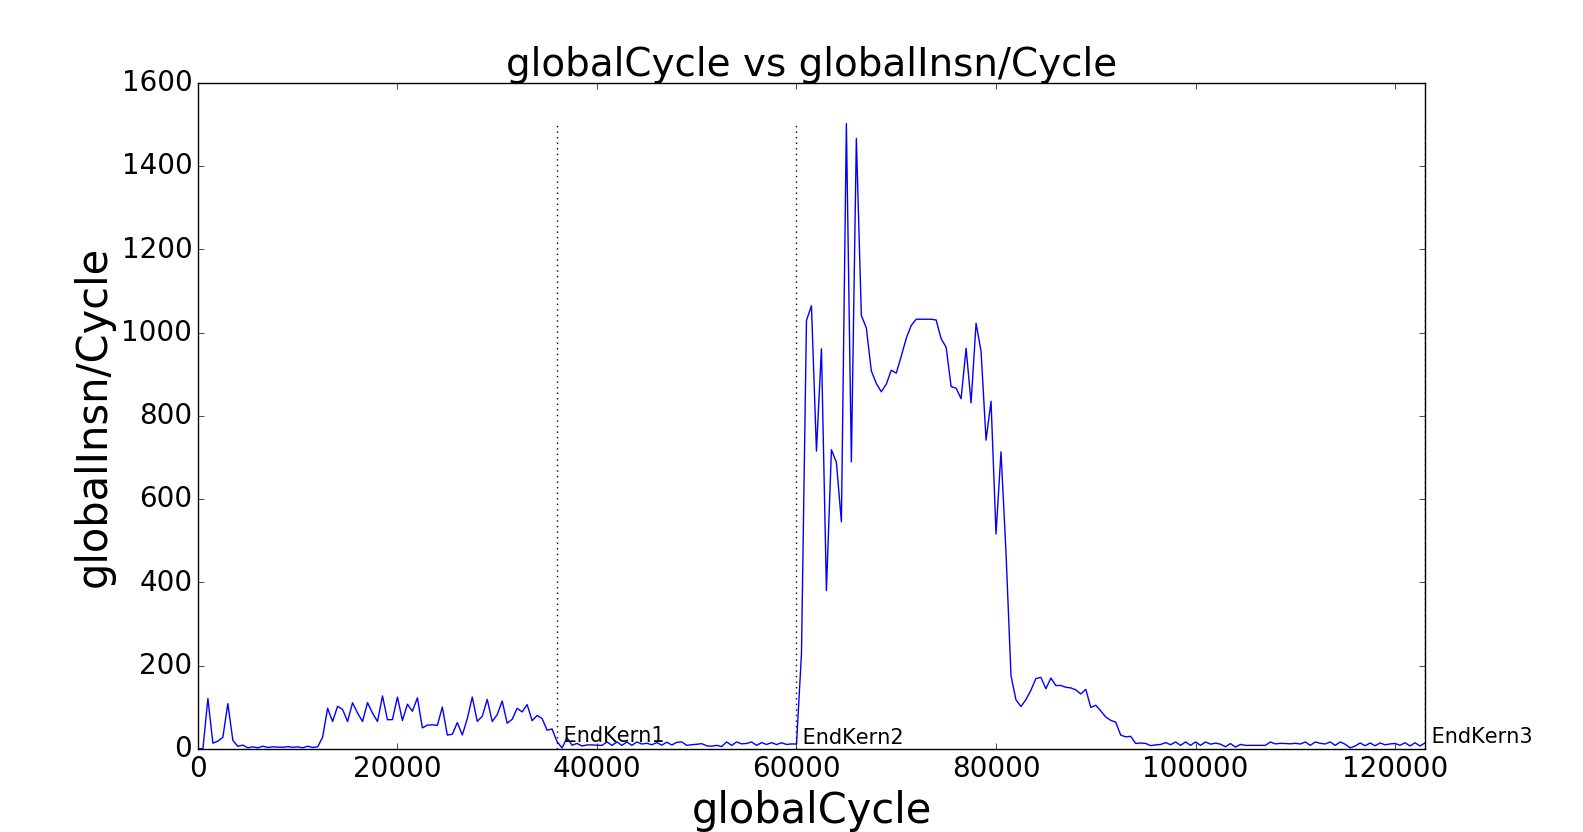}
\caption{Forward Convolution (FFT Tiling) Global IPC Plot}
\label{fig:dram_gemm}
\end{figure}

\begin{figure}[h]
\includegraphics[width=\linewidth]{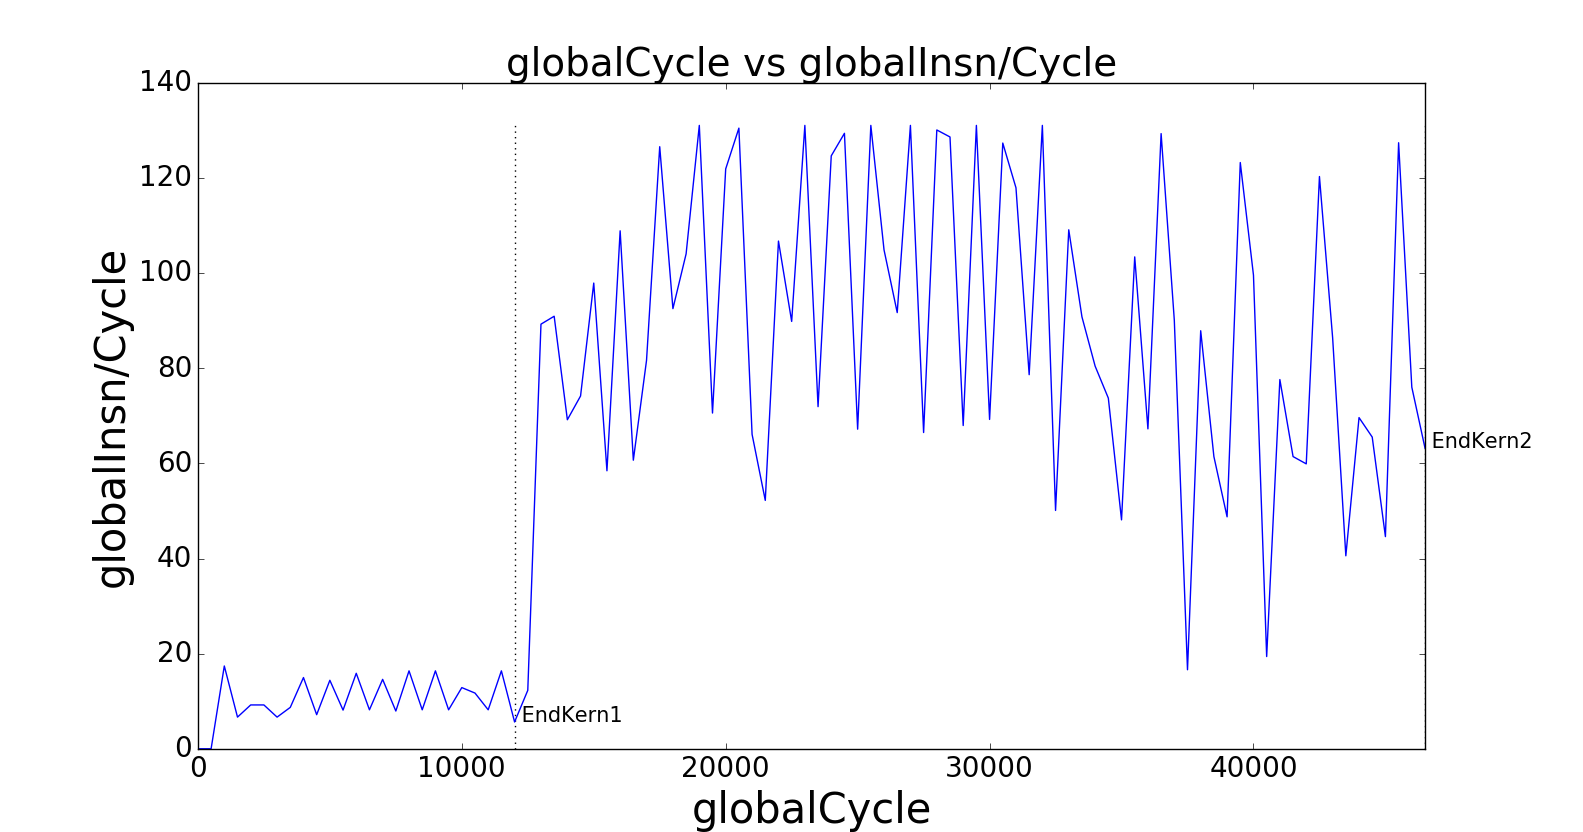}
\caption{Forward Convolution (Winograd) Global IPC Plot}
\label{fig:dram_gemm}
\end{figure}

\begin{figure}[h]
\includegraphics[width=\linewidth]{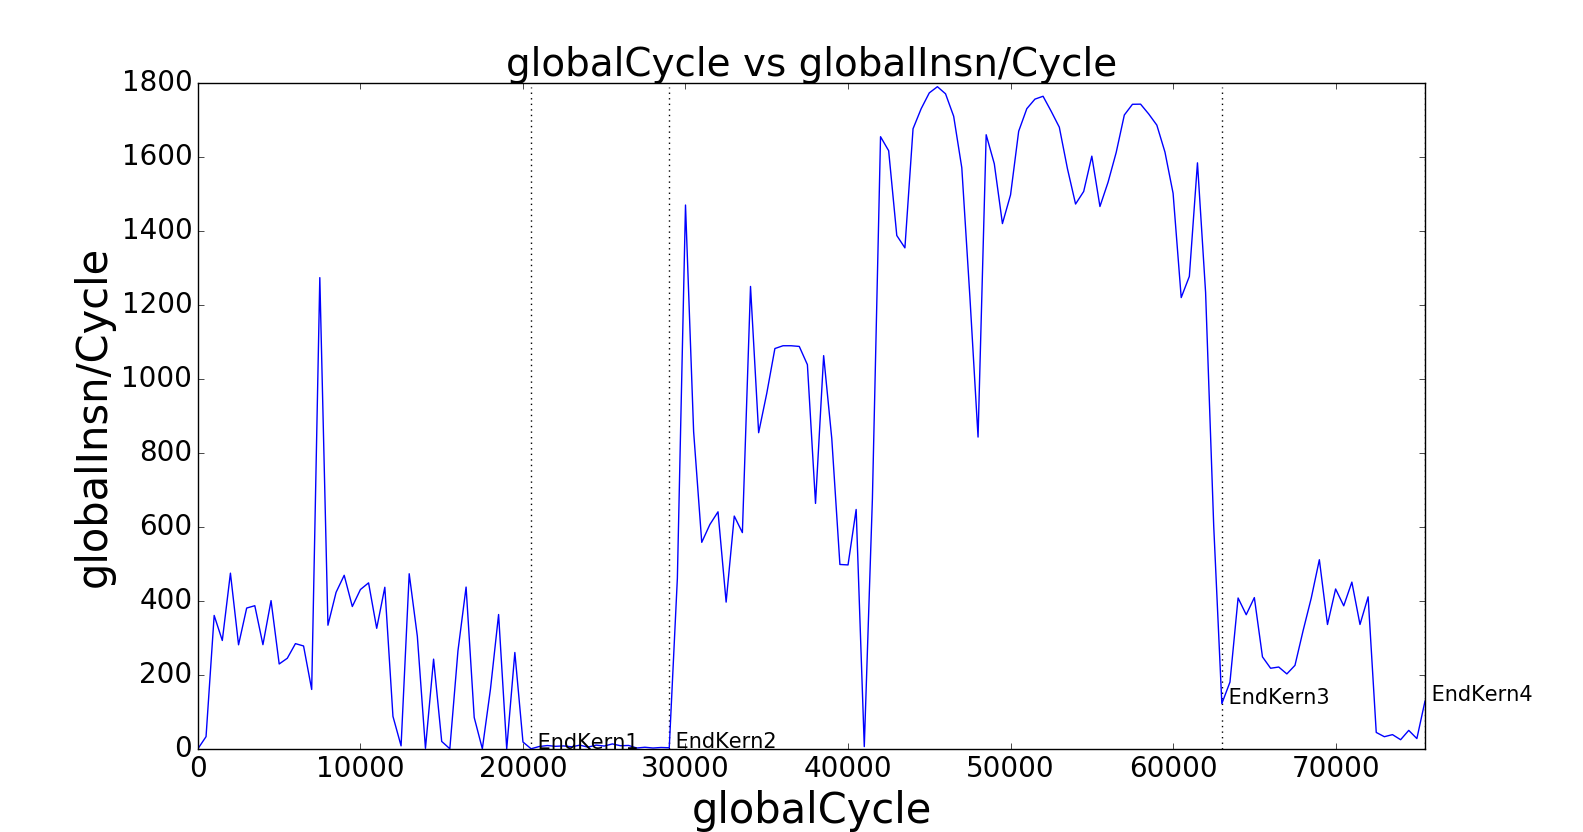}
\caption{Forward Convolution (Winograd Non Fused) Global IPC Plot}
\label{fig:dram_gemm}
\end{figure}

\begin{figure}[h]
\includegraphics[width=\linewidth]{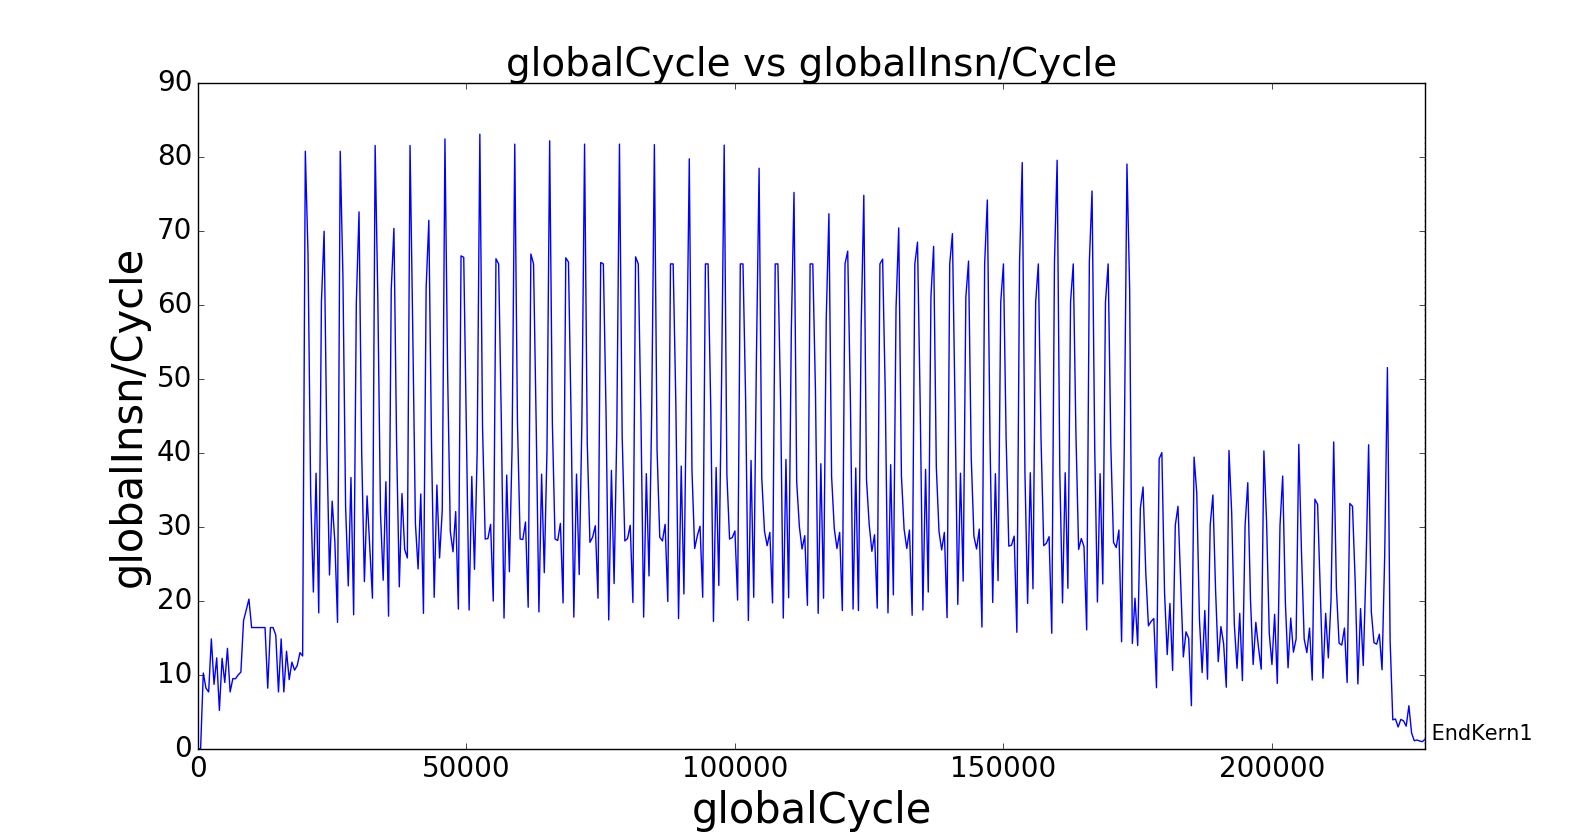}
\caption{Backward Filter Convolution (Algorithm 0) Global IPC Plot}
\label{fig:dram_gemm}
\end{figure}

\begin{figure}[h]
\includegraphics[width=\linewidth]{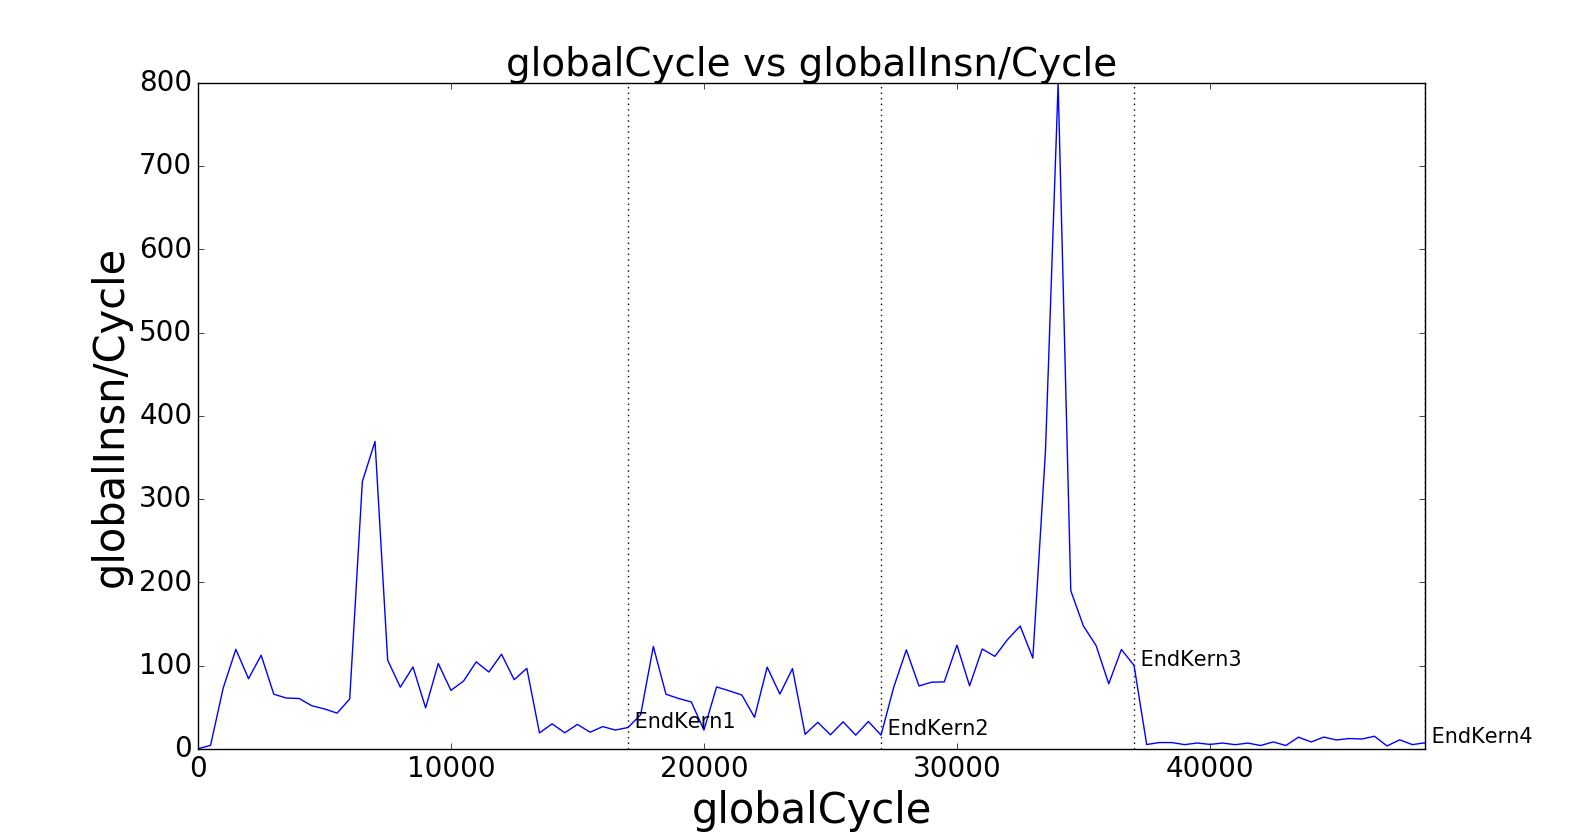}
\caption{Backward Filter Convolution (Winograd Non Fused) Global IPC Plot}
\label{fig:dram_gemm}
\end{figure}

\end{appendix}
